# Supplementary material for: Illuminating the Unseen: Investigating the Context-induced Harms in Behavioral Sensing
Source: arXiv:2404.14665 source file (2024-05-06)
Supplement: Supplementary file 2 [file tab_acc_w_t_demo_appendix.tex]

\begin{table}[htb!]

   \resizebox{0.8\textwidth}{!}{\begin{tabular}{|l|l|rr|rr|rr|rr|}\hline
&& \multicolumn{2}{c|}{\cellcolor[HTML]{CCCCCC}\textbf{DS1 (2018)}}        & \multicolumn{2}{c|}{\cellcolor[HTML]{CCCCCC}\textbf{DS2 (2019)}}        & \multicolumn{2}{c|}{\cellcolor[HTML]{CCCCCC}\textbf{DS3 (2020)}}        & \multicolumn{2}{c|}{\cellcolor[HTML]{CCCCCC}\textbf{DS4 (2021)}}        \\\cline{3-10}
\multirow{-2}{*}{}& \multirow{-2}{*}{\textbf{Sensitive Sub-attributes}} & \multicolumn{1}{c}{p values}  & \multicolumn{1}{c|}{q values}  & \multicolumn{1}{c}{p values}  & \multicolumn{1}{c|}{q values}  & \multicolumn{1}{c}{p values}  & \multicolumn{1}{c|}{q values}  & \multicolumn{1}{c}{p values}  & \multicolumn{1}{c|}{q values}  \\\hline
& First-gen College Student & \cellcolor[HTML]{F4CCCC}0.034 & \cellcolor[HTML]{F4CCCC}0.044 & \cellcolor[HTML]{EA9999}0.001 & \cellcolor[HTML]{F4CCCC}0.022 & 0.507& 0.056& \cellcolor[HTML]{F4CCCC}0.013 & \cellcolor[HTML]{F4CCCC}0.022 \\
& Father's Education& \cellcolor[HTML]{EA9999}0.003 & \cellcolor[HTML]{F4CCCC}0.022 & \cellcolor[HTML]{E06666}0.000 & \cellcolor[HTML]{F4CCCC}0.011 & 0.320& 0.022& 0.167& 0.044\\
& Mother's Education& 0.112& 0.078& \cellcolor[HTML]{EA9999}0.005 & \cellcolor[HTML]{F4CCCC}0.044 & 0.052& 0.011& \cellcolor[HTML]{F4CCCC}0.010 & \cellcolor[HTML]{F4CCCC}0.011 \\
& Gender           & 0.063& 0.056& \cellcolor[HTML]{EA9999}0.004 & \cellcolor[HTML]{F4CCCC}0.033 & 0.785& 0.089& 0.718& 0.089\\
& Immigration Status& 0.087& 0.067& 0.852& 0.078& 0.426& 0.044& 0.628& 0.078\\
& Asian            & \cellcolor[HTML]{F4CCCC}0.015 & \cellcolor[HTML]{F4CCCC}0.033 & 0.095& 0.056& 1.000& 0.100& 0.783& 0.100\\
& Biracial         & 0.899& 0.100& 0.942& 0.100& 0.341& 0.033& 0.482& 0.056\\
& White            & \cellcolor[HTML]{E06666}0.000 & \cellcolor[HTML]{F4CCCC}0.011 & 0.433& 0.067& 0.609& 0.067& 0.114& 0.033\\
\multirow{-9}{*}{Wahle \etal \cite{wahle2016mobile}}              & Sexual Orientation& 0.255& 0.089& 0.858& 0.089& 0.684& 0.078& 0.537& 0.067\\\hline
& First-gen College Student & \cellcolor[HTML]{E06666}0.000 & \cellcolor[HTML]{F4CCCC}0.011 & \cellcolor[HTML]{EA9999}0.002 & \cellcolor[HTML]{F4CCCC}0.022 & 0.079& 0.022& \cellcolor[HTML]{EA9999}0.007 & \cellcolor[HTML]{F4CCCC}0.022 \\
& Father's Education& \cellcolor[HTML]{EA9999}0.002 & \cellcolor[HTML]{F4CCCC}0.044 & \cellcolor[HTML]{EA9999}0.003 & \cellcolor[HTML]{F4CCCC}0.033 & 0.678& 0.078& 0.382& 0.089\\
& Mother's Education& \cellcolor[HTML]{EA9999}0.004 & 0.056& 0.444& 0.100& 0.067& 0.011& \cellcolor[HTML]{F4CCCC}0.010 & \cellcolor[HTML]{F4CCCC}0.033 \\
& Gender           & 0.305& 0.089& \cellcolor[HTML]{EA9999}0.005 & \cellcolor[HTML]{F4CCCC}0.044 & 0.247& 0.044& 0.083& 0.056\\
& Immigration Status& \cellcolor[HTML]{EA9999}0.001 & \cellcolor[HTML]{F4CCCC}0.022 & \cellcolor[HTML]{EA9999}0.001 & \cellcolor[HTML]{F4CCCC}0.011 & 0.507& 0.067& 0.362& 0.078\\
& Asian            & \cellcolor[HTML]{EA9999}0.005 & 0.067& \cellcolor[HTML]{F4CCCC}0.012 & 0.067& 0.886& 0.089& 0.806& 0.100\\
& Biracial         & 0.959& 0.100& 0.129& 0.078& 0.130& 0.033& 0.338& 0.067\\
& White            & \cellcolor[HTML]{EA9999}0.001 & \cellcolor[HTML]{F4CCCC}0.033 & \cellcolor[HTML]{EA9999}0.009 & 0.056& 0.892& 0.100& 0.075& 0.044\\
\multirow{-9}{*}{Saeb \etal \cite{saeb2015mobile}}               & Sexual Orientation& 0.138& 0.078& 0.292& 0.089& 0.406& 0.056& \cellcolor[HTML]{EA9999}0.003 & \cellcolor[HTML]{F4CCCC}0.011 \\\hline
& First-gen College Student & \cellcolor[HTML]{F4CCCC}0.034 & \cellcolor[HTML]{F4CCCC}0.044 & \cellcolor[HTML]{EA9999}0.001 & \cellcolor[HTML]{F4CCCC}0.011 & 0.180& 0.033& \cellcolor[HTML]{E06666}0.000 & \cellcolor[HTML]{F4CCCC}0.011 \\
& Father's Education& \cellcolor[HTML]{EA9999}0.003 & \cellcolor[HTML]{F4CCCC}0.022 & \cellcolor[HTML]{EA9999}0.004 & \cellcolor[HTML]{F4CCCC}0.033 & 0.758& 0.089& 0.072& 0.067\\
& Mother's Education& 0.112& 0.078& 0.269& 0.089& 0.273& 0.044& \cellcolor[HTML]{EA9999}0.001 & \cellcolor[HTML]{F4CCCC}0.022 \\
& Gender           & 0.063& 0.056& \cellcolor[HTML]{EA9999}0.001 & \cellcolor[HTML]{F4CCCC}0.022 & 0.161& 0.022& \cellcolor[HTML]{F4CCCC}0.031 & \cellcolor[HTML]{F4CCCC}0.044 \\
& Immigration Status& 0.087& 0.067& \cellcolor[HTML]{F4CCCC}0.019 & \cellcolor[HTML]{F4CCCC}0.044 & 0.952& 0.100& 0.631& 0.089\\
& Asian            & \cellcolor[HTML]{F4CCCC}0.015 & \cellcolor[HTML]{F4CCCC}0.033 & 0.189& 0.067& \cellcolor[HTML]{F4CCCC}0.044 & 0.011& 0.945& 0.100\\
& Biracial         & 0.899& 0.100& 0.085& 0.056& 0.672& 0.078& 0.606& 0.078\\
& White            & \cellcolor[HTML]{E06666}0.000 & \cellcolor[HTML]{F4CCCC}0.011 & 0.657& 0.100& 0.274& 0.056& 0.069& 0.056\\
\multirow{-9}{*}{Canzian \etal \cite{canzian2015trajectories}}            & Sexual Orientation& 0.255& 0.089& 0.222& 0.078& 0.622& 0.067& \cellcolor[HTML]{EA9999}0.007 & \cellcolor[HTML]{F4CCCC}0.033 \\\hline

& First-gen College Student & \cellcolor[HTML]{F4CCCC}0.033 & \cellcolor[HTML]{F4CCCC}0.033 & \cellcolor[HTML]{EA9999}0.002 & \cellcolor[HTML]{F4CCCC}0.022 & 0.183& 0.067& \cellcolor[HTML]{EA9999}0.007 & \cellcolor[HTML]{F4CCCC}0.022 \\
& Father's Education& \cellcolor[HTML]{EA9999}0.008 & \cellcolor[HTML]{F4CCCC}0.022 & \cellcolor[HTML]{EA9999}0.002 & \cellcolor[HTML]{F4CCCC}0.033 & 0.184& 0.078& 0.067& 0.056\\
& Mother's Education& 0.441& 0.078& 0.389& 0.100& \cellcolor[HTML]{F4CCCC}0.027 & 0.022& \cellcolor[HTML]{F4CCCC}0.012 & \cellcolor[HTML]{F4CCCC}0.033 \\
& Gender           & 0.277& 0.056& \cellcolor[HTML]{EA9999}0.003 & \cellcolor[HTML]{F4CCCC}0.044 & 0.358& 0.089& 0.093& 0.067\\
& Immigration Status& \cellcolor[HTML]{EA9999}0.006 & \cellcolor[HTML]{F4CCCC}0.011 & \cellcolor[HTML]{EA9999}0.001 & \cellcolor[HTML]{F4CCCC}0.011 & \cellcolor[HTML]{F4CCCC}0.026 & 0.011& 0.889& 0.100\\
& Asian            & 0.750& 0.089& \cellcolor[HTML]{EA9999}0.009 & 0.056& 0.670& 0.100& 0.793& 0.089\\
& Biracial         & 0.930& 0.100& 0.140& 0.078& 0.136& 0.056& 0.291& 0.078\\
& White            & 0.202& 0.044& \cellcolor[HTML]{F4CCCC}0.012 & 0.067& 0.063& 0.033& 0.060& 0.044\\
\multirow{-9}{*}{Wang \etal \cite{wang2018tracking}}               & Sexual Orientation& 0.309& 0.067& 0.307& 0.089& 0.064& 0.044& \cellcolor[HTML]{EA9999}0.001 & \cellcolor[HTML]{F4CCCC}0.011 \\\hline
& First-gen College Student & 0.239& 0.056& 0.180& 0.044& 0.211& 0.033& 0.447& 0.067\\
& Father's Education& 0.277& 0.067& 0.991& 0.100& 0.298& 0.056& 0.215& 0.011\\
& Mother's Education& \cellcolor[HTML]{F4CCCC}0.023 & 0.011& 0.116& 0.011& 0.991& 0.100& 0.269& 0.033\\
& Gender           & 0.172& 0.033& 0.256& 0.056& 0.607& 0.078& 0.216& 0.022\\
& Immigration Status& 0.219& 0.044& 0.642& 0.089& 0.506& 0.067& 0.978& 0.100\\
& Asian            & 0.718& 0.100& 0.161& 0.033& \cellcolor[HTML]{F4CCCC}0.021 & \cellcolor[HTML]{F4CCCC}0.022 & 0.342& 0.044\\
& Biracial         & 0.574& 0.089& 0.148& 0.022& \cellcolor[HTML]{EA9999}0.001 & \cellcolor[HTML]{F4CCCC}0.011 & 0.739& 0.089\\
& White            & 0.151& 0.022& 0.256& 0.067& 0.275& 0.044& 0.542& 0.078\\
\multirow{-9}{*}{Xu \etal - Interpretable \cite{xu2019leveraging}} & Sexual Orientation& 0.330& 0.078& 0.556& 0.078& 0.838& 0.089& 0.392& 0.056\\\hline
& First-gen College Student & 0.548& 0.044& 0.058& 0.044& 0.696& 0.056& 0.294& 0.044\\
& Father's Education& 0.737& 0.078& 0.603& 0.089& 0.910& 0.089& 0.975& 0.100\\
& Mother's Education& 0.564& 0.056& 0.580& 0.067& 0.319& 0.033& 0.681& 0.078\\
& Gender           & 0.355& 0.022& 0.313& 0.056& 0.910& 0.089& 0.842& 0.089\\
& Immigration Status& 0.742& 0.089& \cellcolor[HTML]{F4CCCC}0.023 & \cellcolor[HTML]{F4CCCC}0.033 & 0.185& 0.022& 0.629& 0.067\\
& Asian            & 0.751& 0.100& \cellcolor[HTML]{EA9999}0.001 & \cellcolor[HTML]{F4CCCC}0.022 & \cellcolor[HTML]{F4CCCC}0.012 & 0.011& 0.171& 0.033\\
& Biracial         & 0.343& 0.011& 0.589& 0.078& 0.855& 0.078& 0.066& 0.022\\
& White            & 0.428& 0.033& \cellcolor[HTML]{EA9999}0.001 & \cellcolor[HTML]{F4CCCC}0.011 & 0.396& 0.044& 0.343& 0.056\\
\multirow{-9}{*}{Xu \etal - Personalized \cite{xu2022survey}}  & Sexual Orientation& 0.658& 0.067& 0.731& 0.100& 0.825& 0.067& 0.066& 0.011\\
& First-gen College Student & 0.826& 0.067& 0.238& 0.044& 0.107& 0.033& \cellcolor[HTML]{F4CCCC}0.027 & 0.011\\\hline
& Father's Education& 0.956& 0.089& 0.750& 0.078& 0.052& 0.022& 0.115& 0.044\\
& Mother's Education& 0.366& 0.044& 0.106& 0.033& \cellcolor[HTML]{F4CCCC}0.038 & 0.011& 0.074& 0.022\\
& Gender           & 0.992& 0.100& 0.916& 0.089& 0.472& 0.067& 0.582& 0.078\\
& Immigration Status& 0.946& 0.078& 0.073& 0.022& 0.812& 0.100& 0.879& 0.100\\
& Asian            & 0.261& 0.033& 0.378& 0.056& 0.645& 0.078& 0.647& 0.089\\
& Biracial         & 0.170& 0.022& 0.057& 0.011& 0.239& 0.044& 0.496& 0.067\\
& White            & 0.654& 0.056& 0.921& 0.100& 0.279& 0.056& 0.090& 0.033\\
\multirow{-9}{*}{Chikersal \etal \cite{chikersal2021detecting}}          & Sexual Orientation& 0.027& 0.011& 0.416& 0.067& 0.660& 0.089& 0.129& 0.056 \\\hline   
\end{tabular}}
\caption{Acc}\label{tab:acc_w_t_demo_appendix}
\end{table}
