# Supplementary material for: Illuminating the Unseen: Investigating the Context-induced Harms in Behavioral Sensing
Source: arXiv:2404.14665 source file (2024-05-06)
Supplement: Supplementary file 3 [file tab_fnr_w_t_demo_appendix.tex]

\begin{table}[htb!]

   \resizebox{0.8\textwidth}{!}{\begin{tabular}{|l|l|rr|rr|rr|rr|}\hline
&& \multicolumn{2}{c|}{\cellcolor[HTML]{CCCCCC}\textbf{DS1 (2018)}}        & \multicolumn{2}{c|}{\cellcolor[HTML]{CCCCCC}\textbf{DS2 (2019)}}        & \multicolumn{2}{c|}{\cellcolor[HTML]{CCCCCC}\textbf{DS3 (2020)}}        & \multicolumn{2}{c|}{\cellcolor[HTML]{CCCCCC}\textbf{DS4 (2021)}}        \\\cline{3-10}
\multirow{-2}{*}{}& \multirow{-2}{*}{\textbf{Sensitive Sub-attributes}} & \multicolumn{1}{c}{p values}  & \multicolumn{1}{c|}{q values}  & \multicolumn{1}{c}{p values}  & \multicolumn{1}{c|}{q values}  & \multicolumn{1}{c}{p values}  & \multicolumn{1}{c|}{q values}  & \multicolumn{1}{c}{p values}  & \multicolumn{1}{c|}{q values}  \\\hline
     & First-gen College Student                  & 1.000& 0.056& 0.155& 0.044& 0.181& 0.022& 0.470& 0.044\\
     & Father's Education& 1.000& 0.056& 0.147& 0.033& 0.687& 0.089& 0.494& 0.067\\
     & Mother's Education& 1.000& 0.056& 0.423& 0.078& 0.576& 0.067& 0.565& 0.078\\
     & Gender            & 1.000& 0.056& 0.128& 0.022& 0.145& 0.011& 0.312& 0.022\\
     & Immigration Status& 1.000& 0.056& 0.228& 0.056& 0.443& 0.044& 0.565& 0.078\\
     & Asian             & 1.000& 0.056& 0.350& 0.067& 0.562& 0.056& 0.080& 0.011\\
     & Biracial          & 1.000& 0.056& 0.739& 0.100& 0.576& 0.067& 0.777& 0.100\\
     & White             & 1.000& 0.056& \cellcolor[HTML]{F4CCCC}0.037 & 0.011& 0.805& 0.100& 0.328& 0.033\\
\multirow{-9}{*}{Wahle \etal \cite{wahle2016mobile}}               & Sexual Orientation& 1.000& 0.056& 0.714& 0.089& 0.255& 0.033& 0.471& 0.056\\\hline
     & First-gen College Student                  & 0.315& 0.056& 1.000& 0.056& 0.452& 0.067& 0.416& 0.067\\
     & Father's Education& \cellcolor[HTML]{F4CCCC}0.016 & \cellcolor[HTML]{F4CCCC}0.022 & 1.000& 0.056& 0.266& 0.044& \cellcolor[HTML]{EA9999}0.004 & \cellcolor[HTML]{F4CCCC}0.022 \\
     & Mother's Education& 0.069& 0.033& 1.000& 0.056& 0.870& 0.100& 0.119& 0.056\\
     & Gender            & 0.113& 0.044& 1.000& 0.056& 0.408& 0.056& 0.635& 0.078\\
     & Immigration Status& 0.381& 0.078& 1.000& 0.056& 0.622& 0.089& 0.074& 0.044\\
     & Asian             & \cellcolor[HTML]{EA9999}0.006 & \cellcolor[HTML]{F4CCCC}0.011 & 1.000& 0.056& 0.550& 0.078& 1.000& 0.100\\
     & Biracial          & 0.726& 0.089& 1.000& 0.056& \cellcolor[HTML]{EA9999}0.009 & \cellcolor[HTML]{F4CCCC}0.022 & \cellcolor[HTML]{EA9999}0.004 & \cellcolor[HTML]{F4CCCC}0.011 \\
     & White             & 0.378& 0.067& 1.000& 0.056& \cellcolor[HTML]{F4CCCC}0.041 & 0.033& 0.060& 0.033\\
\multirow{-9}{*}{Saeb \etal \cite{saeb2015mobile}}                 & Sexual Orientation& 0.804& 0.100& 1.000& 0.056& \cellcolor[HTML]{EA9999}0.004 & \cellcolor[HTML]{F4CCCC}0.011 & 0.939& 0.089\\\hline
%      & First-gen College Student                  & 0.369& 0.056& 0.111& 0.022& 0.503& 0.044& 0.601& 0.078\\
%      & Father's Education& 0.083& 0.022& 0.470& 0.078& 0.728& 0.078& 0.408& 0.067\\
%      & Mother's Education& 0.302& 0.044& 0.386& 0.067& 0.519& 0.056& \cellcolor[HTML]{F4CCCC}0.025 & 0.011\\
%      & Gender            & 0.796& 0.089& 0.381& 0.056& 0.605& 0.067& 0.187& 0.033\\
%      & Immigration Status& 0.208& 0.033& 0.371& 0.044& \cellcolor[HTML]{F4CCCC}0.038 & 0.011& 0.289& 0.044\\
%      & Asian             & 0.752& 0.078& \cellcolor[HTML]{EA9999}0.003 & \cellcolor[HTML]{F4CCCC}0.011 & 0.223& 0.022& 0.704& 0.089\\
%      & Biracial          & 0.739& 0.067& 0.975& 0.100& 0.777& 0.089& 0.346& 0.056\\
%      & White             & 0.861& 0.100& 0.858& 0.089& 0.307& 0.033& 0.141& 0.022\\
% \multirow{-9}{*}{Farhan \etal \cite{farhan2016behavior}}           & Sexual Orientation& \cellcolor[HTML]{F4CCCC}0.049 & 0.011& 0.230& 0.033& 0.878& 0.100& 0.715& 0.100\\\hline
     & First-gen College Student                  & 1.000& 0.056& 0.200& 0.044& 0.731& 0.067& 0.068& 0.033\\
     & Father's Education& 1.000& 0.056& 0.898& 0.089& 0.108& 0.011& 0.847& 0.100\\
     & Mother's Education& 1.000& 0.056& \cellcolor[HTML]{F4CCCC}0.016 & 0.011& 0.173& 0.022& 0.070& 0.044\\
     & Gender            & 1.000& 0.056& \cellcolor[HTML]{F4CCCC}0.036 & 0.022& 0.211& 0.033& 0.070& 0.044\\
     & Immigration Status& 1.000& 0.056& 0.092& 0.033& 0.682& 0.056& \cellcolor[HTML]{F4CCCC}0.049 & 0.022\\
     & Asian             & 1.000& 0.056& 0.949& 0.100& 0.769& 0.078& 0.614& 0.089\\
     & Biracial          & 1.000& 0.056& 0.485& 0.067& 0.855& 0.100& 0.559& 0.078\\
     & White             & 1.000& 0.056& 0.590& 0.078& 0.819& 0.089& \cellcolor[HTML]{F4CCCC}0.024 & 0.011\\
\multirow{-9}{*}{Canzian \etal \cite{canzian2015trajectories}}     & Sexual Orientation& 1.000& 0.056& 0.228& 0.056& 0.342& 0.044& 0.401& 0.067\\\hline
     & First-gen College Student                  & 0.647& 0.067& 1.000& 0.056& 0.692& 0.078& 0.213& 0.022\\
     & Father's Education& 0.403& 0.056& 1.000& 0.056& 0.892& 0.100& 0.650& 0.078\\
     & Mother's Education& 0.928& 0.100& 1.000& 0.056& 0.312& 0.044& 0.577& 0.067\\
     & Gender            & 0.268& 0.033& 1.000& 0.056& 0.429& 0.056& 0.703& 0.089\\
     & Immigration Status& 0.715& 0.078& 1.000& 0.056& 0.622& 0.067& 0.768& 0.100\\
     & Asian             & 0.302& 0.044& 1.000& 0.056& 0.216& 0.022& 0.177& 0.011\\
     & Biracial          & \cellcolor[HTML]{F4CCCC}0.032 & 0.011& 1.000& 0.056& 0.693& 0.089& 0.418& 0.044\\
     & White             & 0.059& 0.022& 1.000& 0.056& 0.310& 0.033& 0.428& 0.056\\
\multirow{-9}{*}{Wang \etal \cite{wang2018tracking}}               & Sexual Orientation& 0.860& 0.089& 1.000& 0.056& 0.145& 0.011& 0.311& 0.033\\\hline
%      & First-gen College Student                  & 0.843& 0.078& 0.529& 0.067& 0.535& 0.089& 0.253& 0.056\\
%      & Father's Education& 0.916& 0.089& 0.704& 0.100& 0.260& 0.056& 0.160& 0.033\\
%      & Mother's Education& \cellcolor[HTML]{EA9999}0.004 & \cellcolor[HTML]{F4CCCC}0.033 & \cellcolor[HTML]{F4CCCC}0.020 & 0.011& 0.535& 0.089& 0.634& 0.078\\
%      & Gender            & \cellcolor[HTML]{EA9999}0.002 & \cellcolor[HTML]{F4CCCC}0.022 & 0.200& 0.033& 0.068& 0.022& 0.624& 0.067\\
%      & Immigration Status& \cellcolor[HTML]{F4CCCC}0.047 & 0.044& 0.392& 0.044& 0.247& 0.044& 0.246& 0.044\\
%      & Asian             & 0.946& 0.100& 0.603& 0.078& \cellcolor[HTML]{F4CCCC}0.050 & 0.011& 0.920& 0.100\\
%      & Biracial          & 0.095& 0.056& 0.512& 0.056& 0.535& 0.089& 0.150& 0.022\\
%      & White             & \cellcolor[HTML]{E06666}0.000 & \cellcolor[HTML]{F4CCCC}0.011 & 0.679& 0.089& 0.186& 0.033& 0.064& 0.011\\
% \multirow{-9}{*}{Lu etal \cite{lu2018joint}}             & Sexual Orientation& 0.218& 0.067& \cellcolor[HTML]{F4CCCC}0.046 & 0.022& 0.301& 0.067& 0.724& 0.089\\\hline
     & First-gen College Student                  & 0.603& 0.078& \cellcolor[HTML]{F4CCCC}0.011 & \cellcolor[HTML]{F4CCCC}0.022 & 0.284& 0.067& 0.953& 0.100\\
     & Father's Education& 0.805& 0.100& 0.723& 0.089& 0.978& 0.100& 0.930& 0.089\\
     & Mother's Education& 0.140& 0.044& 0.482& 0.078& \cellcolor[HTML]{EA9999}0.004 & \cellcolor[HTML]{F4CCCC}0.022 & 0.051& 0.011\\
     & Gender            & \cellcolor[HTML]{F4CCCC}0.033 & 0.011& \cellcolor[HTML]{EA9999}0.003 & \cellcolor[HTML]{F4CCCC}0.011 & 0.095& 0.033& 0.142& 0.033\\
     & Immigration Status& 0.578& 0.067& 0.336& 0.067& 0.575& 0.078& 0.099& 0.022\\
     & Asian             & 0.081& 0.033& 0.779& 0.100& 0.217& 0.056& 0.561& 0.067\\
     & Biracial          & 0.711& 0.089& 0.166& 0.044& 0.095& 0.033& 0.207& 0.056\\
     & White             & 0.252& 0.056& 0.294& 0.056& 0.736& 0.089& 0.146& 0.044\\
\multirow{-9}{*}{Xu \etal - Interpretable \cite{xu2019leveraging}} & Sexual Orientation& 0.080& 0.022& 0.091& 0.033& \cellcolor[HTML]{E06666}0.000 & \cellcolor[HTML]{F4CCCC}0.011 & 0.812& 0.078\\\hline
     & First-gen College Student                  & 0.912& 0.089& 0.866& 0.100& \cellcolor[HTML]{F4CCCC}0.027 & 0.011& 0.361& 0.044\\
     & Father's Education& 0.320& 0.044& 0.122& 0.033& 0.743& 0.100& \cellcolor[HTML]{EA9999}0.005 & \cellcolor[HTML]{F4CCCC}0.011 \\
     & Mother's Education& 0.335& 0.056& 0.400& 0.067& 0.604& 0.089& 0.239& 0.033\\
     & Gender            & 0.548& 0.067& 0.307& 0.044& 0.207& 0.056& 0.074& 0.022\\
     & Immigration Status& 0.844& 0.078& 0.719& 0.078& 0.376& 0.078& 0.654& 0.056\\
     & Asian             & 0.149& 0.033& 0.831& 0.089& 0.195& 0.044& 0.927& 0.078\\
     & Biracial          & \cellcolor[HTML]{EA9999}0.009 & \cellcolor[HTML]{F4CCCC}0.011 & \cellcolor[HTML]{EA9999}0.006 & \cellcolor[HTML]{F4CCCC}0.011 & \cellcolor[HTML]{F4CCCC}0.027 & 0.011& 0.995& 0.100\\
     & White             & 0.060& 0.022& 0.316& 0.056& 0.075& 0.033& 0.661& 0.067\\
\multirow{-9}{*}{Xu \etal - Personalized \cite{xu2022survey}}      & Sexual Orientation& 0.942& 0.100& 0.107& 0.022& 0.228& 0.067& 0.981& 0.089\\\hline
     & First-gen College Student                  & 0.745& 0.067& 0.426& 0.056& 0.682& 0.078& \cellcolor[HTML]{F4CCCC}0.019 & 0.011\\
     & Father's Education& \cellcolor[HTML]{EA9999}0.002 & \cellcolor[HTML]{F4CCCC}0.011 & 0.169& 0.033& 0.978& 0.089& 0.598& 0.100\\
     & Mother's Education& 0.727& 0.056& 0.965& 0.100& 0.991& 0.100& 0.081& 0.056\\
     & Gender            & 0.892& 0.100& 0.875& 0.089& 0.380& 0.067& 0.140& 0.067\\
     & Immigration Status& 0.831& 0.078& 0.841& 0.078& 0.327& 0.056& \cellcolor[HTML]{F4CCCC}0.029 & 0.022\\
     & Asian             & 0.872& 0.089& 0.288& 0.044& 0.095& 0.022& 0.509& 0.089\\
     & Biracial          & 0.391& 0.033& 0.118& 0.022& \cellcolor[HTML]{F4CCCC}0.019 & 0.011& 0.055& 0.033\\
     & White             & 0.628& 0.044& \cellcolor[HTML]{F4CCCC}0.016 & 0.011& 0.140& 0.033& 0.486& 0.078\\
\multirow{-9}{*}{Chikersal \etal \cite{chikersal2021detecting}}    & Sexual Orientation& 0.335& 0.022& 0.778& 0.067& 0.283& 0.044& 0.072& 0.044     \\\hline
\end{tabular}}\label{tab_fnr_w_t_demo_appendix}
\caption{FNR.}
\end{table}
