# Supplementary material for: Illuminating the Unseen: Investigating the Context-induced Harms in Behavioral Sensing
Source: arXiv:2404.14665 source file (2024-05-06)
Supplement: Supplementary file 5 [file tab_example_appendix.tex]

\begin{table}[htb!]
\caption{Detailed Information for the example on the disparities in accuracy, false negative rate, and false positive rate. PID stands for participant ID. The ``Protected Group'' column indicates whether the participant belongs to the protected group (Yes) or the unprotected group (No). In total, there are 30 participants, with 10 individuals belonging to the protected group and 20 individuals from the unprotected group. A value of 1 is assigned to cases where the algorithm accurately predicted the ground truth and a value of 0 is assigned to cases where the algorithm did not accurately predict the ground truth.}
   \resizebox{0.5\textwidth}{!}
{\begin{tabular}{ccccc}\hline
PID & True Label & Prediction & Protected Group & Assigned Value \\\hline
1& 1 & 0 & Yes & 0 \\
2 & 1 & 1 & Yes & 1 \\
3 & 1 & 1 & No  & 1 \\
4 & 0 & 0 & No  & 1 \\
5 & 0 & 0 & No  & 1 \\
6 & 1 & 1 & No  & 1 \\
7 & 1 & 1 & No  & 1 \\
8 & 0 & 1 & Yes & 0 \\
9 & 0 & 0 & Yes & 1 \\
10 & 1 & 0 & Yes & 0 \\
11 & 0 & 1 & No  & 0 \\
12 & 0 & 0 & Yes & 1 \\
13 & 1 & 0 & Yes & 0 \\
14 & 1 & 1 & No  & 1 \\
15 & 0 & 0 & No  & 1 \\
16 & 0 & 0 & No  & 1 \\
17 & 0 & 0 & No  & 1 \\
18 & 0 & 0 & No  & 1 \\
19 & 0 & 1 & No  & 0 \\
20 & 0 & 0 & No  & 1 \\
21 & 1 & 1 & No  & 1 \\
22 & 1 & 0 & Yes & 0 \\
23 & 0 & 0 & No  & 1 \\
24 & 0 & 0 & No  & 1 \\
25 & 0 & 0 & No  & 1 \\
26 & 0 & 0 & No  & 1 \\
27 & 0 & 0 & No  & 1 \\
28 & 1 & 0 & No  & 0 \\
29 & 1 & 0 & Yes & 0 \\
30 & 0 & 0 & Yes & 1\\\hline
\end{tabular}}
\label{tab:appendix_example}
\end{table}
